# Supplementary material for: Natural Language Does Not Emerge 'Naturally' in Multi-Agent Dialog
Source: arXiv:1706.08502 source file (2017-08-20)
Supplement: Supplementary file 1 [file supp.tex]

% \sk{
% Things to-do for supplement:
% \begin{compactenum}
% \item \sout{larger language chart with more examples}
% \item \sout{complete task encoding table for concept vocabulary}
% \item figure to explain the task, synthetic world  (defer?)
% \item \sout{example conversation (similar to iccv)}
% \item Explain how we obtain the dialog tree trends
% \item \sout{implementation details}
% \item \sout{conditional grounding tables for memoryless A and Q}
% \item 12 a vocab memoryless, interesting trends (defer?)
% \item \sout{example of a dialog tree}
% \item REINFORCE equations and derivations
% \item \sout{Overview table containing detail of summary}
% \end{compactenum}}
%%%%%%%%%%%%%%%%%%%%%%%%%%%%%%%%%%%%%%%%%%%%%%%%%%%%%%%%
\onecolumn
\section*{Supplement}
% \sk{
% The supplement is organized as follows:
% \begin{compactitem}
% 	\item \refsec{sec:overview_supp} overviews all the settings characterizing communication language between the agents.
%     %\item \refsec{sec:grounding_supp} gives details of learnt grounding in two important settings,
%     \item \refsec{sec:dialog_trees_supp} describes the structure and construction of dialog trees,
%     \item Finally, \refsec{sec:lang_evolution_supp} builds on dialog trees and details the procedure to obtain a timeline of how the agents learn grounding for symbols at intermediate stages of training.
% \end{compactitem}}
\sk{
The supplement contains:
(a) An overview of all settings characterizing the communication language learnt by the agents (\reftab{tab:overview-setting-elaborate}),
(b) A detailed evolution of language chart, highlighting all `concepts' grounded at various times during training (\reffig{fig:lang_chart_supp}).}

%%%%%%%%%%%%%%%%%%%%%%%%%%%%%%%%%%%%%%%%%%%%%%%%
\begin{table*}[h]
	\centering
    \begin{tabu}{p{1in} c c c c c c}
    	\toprule
        \multirow{2}{*}{Setting} 
    	& \multicolumn{2}{c}{Vocab.} 
        & \multicolumn{2}{c}{Memory} 
        & \multirow{2}{*}{Gen.}
        & \multirow{2}{*}{Characteristics}\\

  	  & \textbf{$V_Q$} & \textbf{$V_A$} & A & Q & & \\ \midrule

    Overcomplete (Sec.4.1 main) & 64 & 64 & \cmark & \cmark & 25.6 \%
    	&  
  		\begin{minipage}[c]{0.5\textwidth}
          \begin{compactitem}
          \item Non-compositional language
          \item \Qbot insignificant
          \item Inconsistent \Abot grounding across rounds
          \item Poor generalization to unseen instances
          \end{compactitem}
        \end{minipage}\\ \\
        %\tabucline[1pt black!30 off 5pt]{-}
        
        Attr-Value (Sec.4.2 main) & 3 & 12 & \cmark & \cmark & 38.5\% 
        &
   		\begin{minipage}[c]{0.5\textwidth}
          \begin{compactitem}
          \item Non-compositional language
          \item \Qbot uses one round to convey task
          \item Inconsistent \Abot grounding across rounds
          \item Poor generalization to unseen instances
          \end{compactitem}
        \end{minipage}\\ \\
        
%         NoMem-L (\FIXME{ref}) & 6 & 12 & \xmark & \cmark & 44.9\% 
%         & 
%         \begin{minipage}[c]{0.5\textwidth}
%           \begin{compactitem}
%           \item Non-compositional language
%           \item \Qbot, \Abot develop unintuitive grounding
%           \item Poor generalization to unseen instances
%           \end{compactitem}
%         \end{minipage}\\ \\
        
%         Mem-Min (\FIXME{ref}) & 3 & 4 & \cmark & \cmark & 41.0\% 
%         & 
%         \begin{minipage}[c]{0.5\textwidth}
%           \begin{compactitem}
%           \item Compositional language
%           \item \Qbot uses both rounds to convey task
%           \item Inconsistent \Abot grounding across rounds
%           \item Good generalization to unseen instances
%           \end{compactitem}
%         \end{minipage}\\ \\
        
        NoMem-Min (Sec.4.3 main) & 3 & 4 & \xmark & \cmark & 74.4\% 
        &
        \begin{minipage}[c]{0.5\textwidth}
          \begin{compactitem}
          \item Compositional language
          \item \Qbot uses both rounds to convey task
          \item Consistent \Abot grounding across rounds
          \item Good generalization to unseen instances
          \end{compactitem}
        \end{minipage}\\ \bottomrule
    \end{tabu}
    \caption{Overview of settings we explore to analyze language learnt by two agents in a cooperative game, \tnt. Compositional language (last row) as the best generalization and consistent token groundings.}
    \label{tab:overview-setting-elaborate}
\end{table*}

\begin{figure*}[h]
	\centering
	\includegraphics[width=0.99\textwidth]{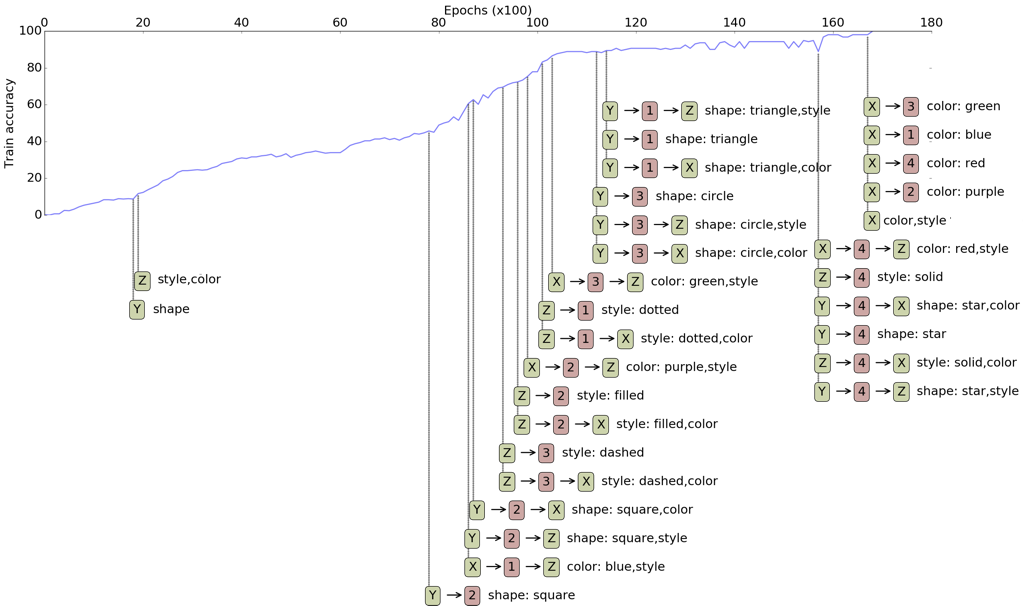}
    \caption{\sk{Detailed timeline for language evolution--captures grounding learnt by the agents during training, overlaid on the accuracy. Note that \Qbot learns encodings for all tasks but \emph{(style, color)}, early (around epoch $20$). Notice how improvement in accuracy is strongly correlated with groundings learnt. Refer text for more details.}}
    \label{fig:lang_chart_supp}
\end{figure*}
