# Supplementary material for: Natural Language Does Not Emerge 'Naturally' in Multi-Agent Dialog
Source: arXiv:1706.08502 source file (2017-08-20)
Supplement: Supplementary file 2 [file all_scenarios_table_elaborate.tex]

%%%%%%%%%%%%%%%%%%%%%%%%%%%%%%%%%%%%%%%%%%%%%%%%
\begin{table*}[h]
	\centering
    \begin{tabu}{p{1in} c c c c c c}
    	\toprule
        \multirow{2}{*}{Setting} 
    	& \multicolumn{2}{c}{Vocab.} 
        & \multicolumn{2}{c}{Memory} 
        & \multirow{2}{*}{Gen.}
        & \multirow{2}{*}{Characteristics}\\

  	  & \textbf{$V_Q$} & \textbf{$V_A$} & A & Q & & \\ \midrule

    Overcomplete (Sec.4.1 main) & 64 & 64 & \cmark & \cmark & 25.6 \%
    	&  
  		\begin{minipage}[c]{0.5\textwidth}
          \begin{compactitem}
          \item Non-compositional language
          \item \Qbot insignificant
          \item Inconsistent \Abot grounding across rounds
          \item Poor generalization to unseen instances
          \end{compactitem}
        \end{minipage}\\ \\
        %\tabucline[1pt black!30 off 5pt]{-}
        
        Attr-Value (Sec.4.2 main) & 3 & 12 & \cmark & \cmark & 38.5\% 
        &
   		\begin{minipage}[c]{0.5\textwidth}
          \begin{compactitem}
          \item Non-compositional language
          \item \Qbot uses one round to convey task
          \item Inconsistent \Abot grounding across rounds
          \item Poor generalization to unseen instances
          \end{compactitem}
        \end{minipage}\\ \\
        
%         NoMem-L (\FIXME{ref}) & 6 & 12 & \xmark & \cmark & 44.9\% 
%         & 
%         \begin{minipage}[c]{0.5\textwidth}
%           \begin{compactitem}
%           \item Non-compositional language
%           \item \Qbot, \Abot develop unintuitive grounding
%           \item Poor generalization to unseen instances
%           \end{compactitem}
%         \end{minipage}\\ \\
        
%         Mem-Min (\FIXME{ref}) & 3 & 4 & \cmark & \cmark & 41.0\% 
%         & 
%         \begin{minipage}[c]{0.5\textwidth}
%           \begin{compactitem}
%           \item Compositional language
%           \item \Qbot uses both rounds to convey task
%           \item Inconsistent \Abot grounding across rounds
%           \item Good generalization to unseen instances
%           \end{compactitem}
%         \end{minipage}\\ \\
        
        NoMem-Min (Sec.4.3 main) & 3 & 4 & \xmark & \cmark & 74.4\% 
        &
        \begin{minipage}[c]{0.5\textwidth}
          \begin{compactitem}
          \item Compositional language
          \item \Qbot uses both rounds to convey task
          \item Consistent \Abot grounding across rounds
          \item Good generalization to unseen instances
          \end{compactitem}
        \end{minipage}\\ \bottomrule
    \end{tabu}
    \caption{Overview of settings we explore to analyze language learnt by two agents in a cooperative game, \tnt. Compositional language (last row) as the best generalization and consistent token groundings.}
    \label{tab:overview-setting-elaborate}
\end{table*}

%%%%%%%%%%%%%%%%%%%%%%%%%%%%%%%%%%%%%%%%%%%%%%%%
% \begin{table*}
% 	\centering
%     \begin{tabular}{c c c c c c c c}
%     	\multirow{2}{*}{Setting} 
%     	& \multicolumn{2}{c}{Vocab.} 
%         & \multicolumn{2}{c}{Memory} 
%         & \multirow{2}{*}{Gen.}
%         & \multirow{2}{*}{Pros}
%         & \multirow{2}{*}{Cons}\\
    
%     & \textbf{$V_Q$} & \textbf{$V_A$} & \Abot & \Qbot &&&\\ \hline
%         Overcomplete (theory) & 6 & 64 & \cmark & \cmark & 0.0\% & blah & blah\\
% 		Large (Sec.\FIXME{ref}) & 6 & 12 & \cmark & \cmark & 24.4\% & blah & blah \\
%         NoMem-Large (Sec.\FIXME{ref}) & 6 & 12 & \xmark & \cmark & xxx & blah & blah \\
%         Mem-Minimal (Sec.\FIXME{ref}) & 3 & 4 & \cmark & \cmark & xxx & blah & blah \\
%         NoMem-Minimal (Sec.\FIXME{ref}) & 3 & 4 & \xmark & \cmark & xxx & blah & blah \\
%         NoMem-Both-Large (Sec.\FIXME{ref}) & 12 & 6 & \xmark & \xmark & xxx & blah & blah \\ \hline
%     \end{tabular}
%     \caption{\FIXME{An overview of all the settings, details in each setting}}
%     \label{tab:overview-setting}
% \end{table*}
